# Supplementary material for: The Story in Your Eyes: An Individual-difference-aware Model for Cross-person Gaze Estimation
Source: arXiv:2106.14183 source file (2021-06-27)
Supplement: Supplementary file 1 [file supp_material.tex]

%%%%%%%%% TITLE
\title{Supplementary Materials}
\maketitle

% %%%%%%%%% TITLE
% \title{Supplementary Materials: \\ The Story in Your Eyes:\\ An Individual-difference-aware Model for Cross-person Gaze Estimation}

% \author{First Author\\
% Institution1\\
% Institution1 address\\
% {\tt\small firstauthor@i1.org}
% % For a paper whose authors are all at the same institution,
% % omit the following lines up until the closing ``}''.
% % Additional authors and addresses can be added with ``\and'',
% % just like the second author.
% % To save space, use either the email address or home page, not both
% \and
% Second Author\\
% Institution2\\
% First line of institution2 address\\
% {\tt\small secondauthor@i2.org}
% }

% \maketitle
% % Remove page # from the first page of camera-ready.

%%%%%%%%% BODY TEXT
In this supplementary material, we include further details on the following:
\begin{itemize}
    \item Details on Person-specific Transform (PT) Module.
    \item Details on definition of the set of affine parameters$~\mathcal{A}$ and random noise$~\mathcal{N}$ in data augmentation procedure for PT training.
    \item Ablation studies on the impact of history length.
    % \item more results on XGaze (+ vm + st trained on XGaze data augment)
\end{itemize}

\section{Person-specific Transform Module}
Our PT Module is a spatial transform network~\cite{NIPS2015_33ceb07b} that consists of a localization net, a grid generator and a sampler. Details of localization net are shown in Tab.~\ref{tbl:pt_model_structure}. 

\begin{table}[b]
  \centering
  \begin{tabular}{c|c|c}
  \hline
             \multicolumn{3}{c}{localization net structure in PT Module~\cite{NIPS2015_33ceb07b}} \\
  \hline
  Layer type & Dimensions & Output (h,w,c) \\
  \hline
  Conv2D & 7 $\times$ 7 & 66,122,8 \\
  Maxpool  & 2 $\times$ 2, stride 2 &  33,61,8 \\
  ReLU & - & 33,61,8 \\
  \hline
  Conv2D & 5 $\times$ 5 &  29,57,12 \\
  Maxpool & 2 $\times$ 2, stride 2 &  14,28,12 \\
  ReLU & - & 14,28,12 \\
  \hline
  Conv2D & 5 $\times$ 5 & 10,24,16 \\
  Maxpool & 2 $\times$ 2, stride 2 & 5,12,16 \\
  ReLU & - & 5,12,16 \\
  \hline
  Linear & 960 $\times$ 32 & 32 \\
  ReLU & - & 32 \\
  Linear & 32 $\times$ 6 & 6 \\

  \hline 
\end{tabular}
  \caption{Summary of the localization net in our PT Module. %In addition, we can see that introducing each module is beneficial for gaze prediction task.
  }
  \label{tbl:pt_model_structure}
\end{table}

\section{Augmentation Parameters for PT Training}
We provide more details on PT training, specially, we would describe the set of parameters$~\mathcal{A}$ for affine transformation and$~\mathcal{N}$ for random noise in Tab.~\ref{tbl:history_heatmap_data_augmentation_parameters}. These parameters are chosen with our experiences. We further demonstrate the generation process step by step in Fig.~\ref{fig:heatmap_demo}. Specifically, the first row shows the process for $r_{t,j}^h$ and the row below is for $\widetilde{r}_{t,j}^h$. For simplicity, we only showcase the scenario where history length is 3. 

To train our PT Module that is both applicable to offline and online case on EVE, we manually set the history length to $4000$ and $8000$ while generating training samples, e.g. size of $\mathcal{H}_{t,j}$ is 4000 and 8000 for each sample. In addition, we uniformly sample one-tenth images from EVE training set instead of using full set. In practice, we will have 25246 training samples on EVE.

% We train the PT Module to predict ground-truth history heatmap $\widetilde{r}_{t,j}^h$ during training, then apply it to predicted $\widetilde{r}_{t,j}^h$ from predicted history heatmap $r_{t,j}^h$ outputted by our Self-Calibration Module. 

% The data augmentation of $\widetilde{r}_{t,j}^h$ is done by applying one affine transformation $a$ to all history samples and random noises $n_k$ to each history sample in $\widetilde{r}_{t,j}^h$.

%Tab.~\ref{tbl:history_heatmap_data_augmentation_parameters} shows our parameters to generate affine transformation set $\mathcal{A}$ and random noise set $\mathcal{N}$, from which $a$ and $n_k$ are randomly chosen. While the length of history can range from 0 to around 15000 time points in EVE dataset, in practice we choose to apply augmentation on fixed history of length 4000 and 8000.
%For each 3 seconds clip in EVE dataset, we randomly select one frame to apply augmentation for three times, which generates a PT training dataset of 25246 samples.

% The parameters are selected by experience in order to generate augmented $\widetilde{r}_{t,j}^h$ that resembles predicted history heatmap $r_{t,j}^h$. 

\begin{table}[b]
  \centering\small
  
% \usepackage{threeparttable}

% \begin{document}

% \begin{table}[! htbp]\centering \caption{Summary Statistics}
% \begin{threeparttable}
% \begin{tabular}{l c c c}
% \toprule\midrule
% \thead{Variable} & \thead{Mean}
%  & \thead{Std. Dev.} & \thead{N}\\ \midrule
% a & a & a\tnote{*} & a \\
% \bottomrule\addlinespace[1ex]
% \end{tabular}
% \begin{tablenotes}\footnotesize
% \item[*] Blahblah
% \end{tablenotes}
% \end{threeparttable}
% \label{table2}
% \end{table}

% \end{document} 

\begin{tabular}{lccc}
  \hline
  Set & Augmentation Type & Distribution & Parameters \\
  \hline
  $\mathcal{A}$  & horizontal scaling &  uniform & [0.7, 1.1] \\
                & vertical scaling &  uniform & [0.4, 1.1] \\
                & rotation & guassian & 0 \pm\ 2$^{\circ}$\\
                & rotation center x & uniform & [-W/3, W/3]$^*$\\
                & rotation center y & uniform & [-H/3, H/3]$^*$\\
  \hline
  
  $\mathcal{N}$  & noise &  guassian & 0 \pm\ 8.4 \\ %0.2^{\circ}\\
  \hline 
\end{tabular}
\\$^*$ W and H are the width and height of the screen.\footnotesize{}

% history_selected = [4000, 8000]
% GUASSIAN_BLUR = (15, 15)
% INPUT_HEATMAP_SIZE = (128, 72)

% def generate_augmentation_params():
%     #scaling uniform  0.7 1.1,  0.4 - 1.1
%     #rotation guassian guassian 0 +- np.pi/60
%     #rotation center univform -960 - 960, -540  -- 540
%     #translation guassian 0 +-  3 * 38.4
    
%     w, h = 1920, 1080
%     scaling = random.uniform(0.8, 1.1), random.uniform(0.7, 1.0)
%     rotation = np.random.normal(0, np.pi/90)
%     rotation_center = random.uniform(-w/3, w/3), random.uniform(-h/3, h/3)
%     translation = np.random.normal(0, 0.0*PIXEL_PER_DEGREE), np.random.normal(0, 0.0*PIXEL_PER_DEGREE)
%     std_random = 0.2*PIXEL_PER_DEGREE
  \caption{Summary of parameters to generate affine transformation set $\mathcal{A}$ and noise set $\mathcal{N}$.}
  \label{tbl:history_heatmap_data_augmentation_parameters}
\end{table}

\begin{table}
  \centering\small
  \begin{tabular}{c|c|c|c}
  \hline
             \multicolumn{4}{c}{Impact of history length on EVE validation set~\cite{Park2020ECCV}} \\
  \hline
  History Length & Gaze Dir. ($^{\circ}$) $\downarrow$ & PoG (cm) $\downarrow$ & PoG (px)  $\downarrow$\\
  \hline
  100 & 3.53 & 4.05 & 140.61 \\  
  200 & 3.32 & 3.80 & 131.98 \\
  500 & 2.95 & 3.38 & 117.40 \\
  1000 & 2.55 & 2.92 & 101.36 \\
  \hline
  2000 & 2.25 & 2.58 & 89.55 \\
  4000 & 2.06 & 2.36 & 82.07 \\
  8000 & 1.95 & 2.22 & 77.08 \\
  \hline
  offline & \textbf{1.89} & \textbf{2.16} & \textbf{74.85}\\  
  \hline 
\end{tabular}

% 100 [('g', 3.5298), ('PoG_px', 140.6093), ('PoG_cm', 4.0495)]
% 200  ('g', 3.3203), ('PoG_px', 131.9837), ('PoG_cm', 3.8011)] 216349
% 500 [('g', 2.9488), ('PoG_px', 117.3977), ('PoG_cm', 3.381)]
% 1000 [('g', 2.5544), ('PoG_px', 101.3631), ('PoG_cm', 2.9192)]
% 2000 [('g', 2.2515), ('PoG_px', 89.5539), ('PoG_cm', 2.5791)]
% 4000 [('g', 2.0672), ('PoG_px', 82.0748), ('PoG_cm', 2.3637)]
% 8000 [('g', 1.9462), ('PoG_px', 77.0835), ('PoG_cm', 2.2199)]
% full  \1.89 & \2.16 & \74.85\\
  \caption{Ablation study of history length on EVE validation set.}
  \label{tbl:history_length_ablation_results_eve}
\end{table}

\begin{figure*}[t]
  \includegraphics[width=1.0\linewidth]{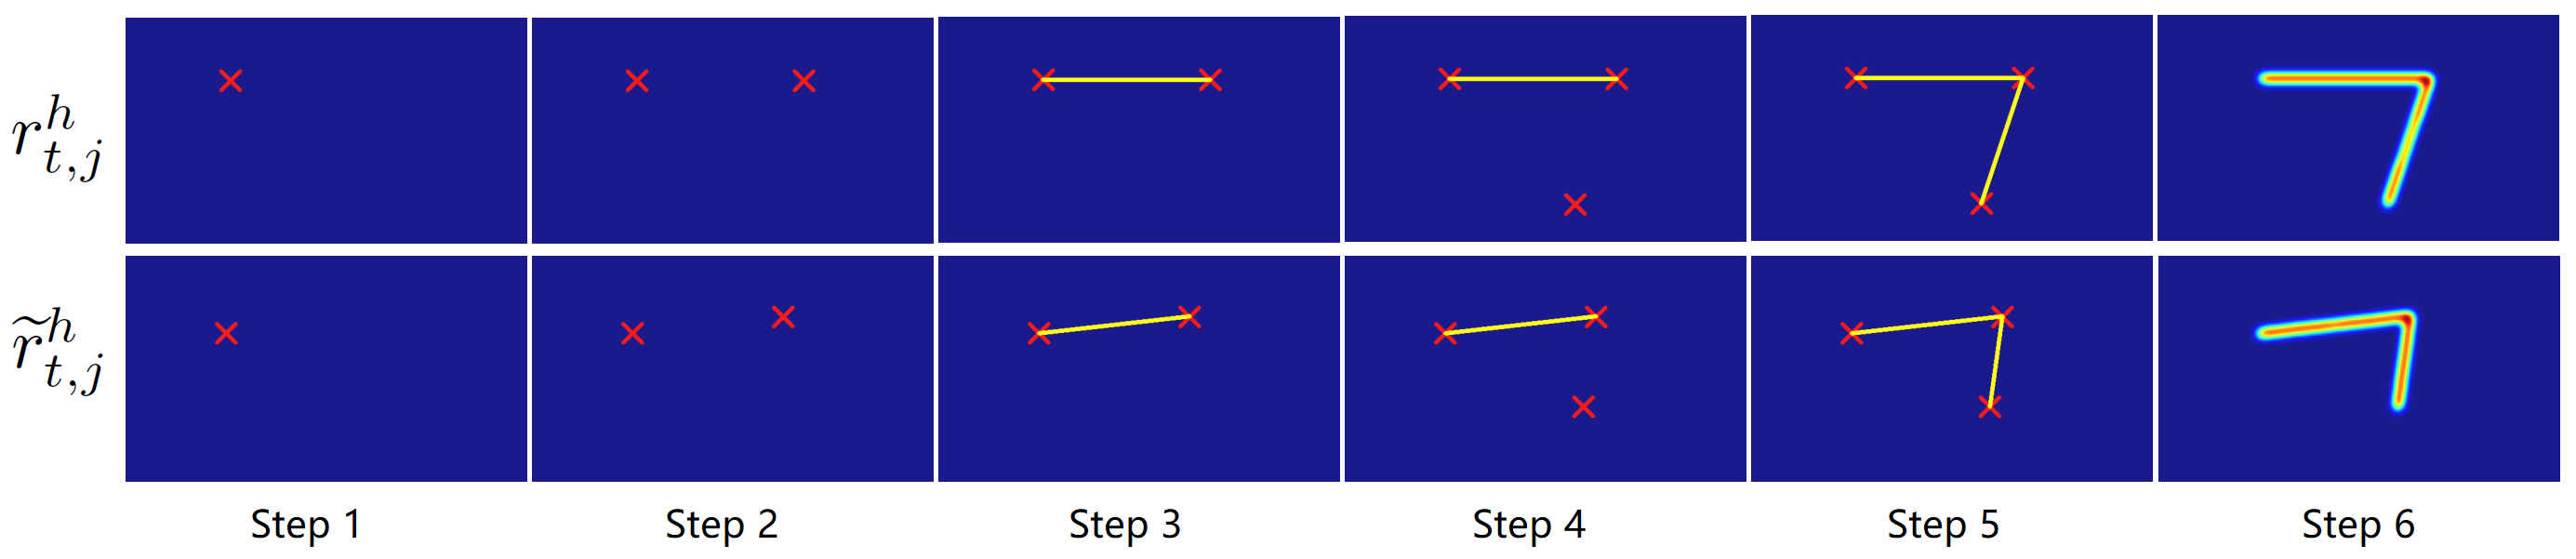}
   %\fbox{\rule{0pt}{1in} \rule{.9\linewidth}{0pt}}
  % \vspace{-0.65cm}
   \caption{
  The generation process for for $r_{t,j}^h$ and $\widetilde{r}_{t,j}^h$ with history length of 3.
   }
   \label{fig:heatmap_demo}
\end{figure*}

% \begin{table*}
%   \centering\small
%   \input{tables/mpii_more}
%   \caption{More results on MPIIGaze~\cite{zhang2017mpiigaze}. We can see that with better InitNet, we are able to further improve the final performance on MPIIGaze.}
%   \label{tbl:more_mpii}
% \end{table*}

\section{Ablation Study: History Length}
Our history prediction map plays an important role in PT Module (See Eq. 4 in our main paper) during training. Intuitively, the longer history from $j$-th person is available, the better performance our PT Module can achieve. To this end, we conduct another experiment on the impact of history length to our proposed method on validation set of EVE~\cite{Park2020ECCV}. Note that data from EVE~\cite{Park2020ECCV} is obtained with free-viewing tasks, e.g. participants would view videos/images/web-pages on screen and they can look at arbitrary location on screen.

We report our results in Tab.~\ref{tbl:history_length_ablation_results_eve}. As can be seen in this table, longer history does lead to better performance on EVE validation set. Interestingly, our InitNet alone gives 2.41$^{\circ}$ performance and compared to various history length, it seems that less than 2000 history length would deteriorate the overall performance. This observation again supports our loss function design that excluding per-sample gaze heatmap ${r}_{t,j}$, which can be taken as an extreme case where only one history sample is available (See Sec. 3.2 in our main paper). 

%learning transformation with per-sample gaze heatmap ${r}_{t,j}$, which can be taken as extreme case with one history sample, is less meaningful as there are only limited information on this heatmap. In addition, focusing on ${r}_{t,j}$ might further confuse the localization net in PT Module.

Please note that we have two settings in our main paper. The online setting receives consecutive frames during test time and do not have access to future frames. And the offline setting assumes all images from the same participants are available during the test time. Our method achieves best results with full history length (i.e., offline), averaged at 10817 for EVE validation set at 10Hz frame rate. Given the observation that less than 2000 samples deteriorate results, we apply our online method on EVE until the history length is greater than 2000.

However, the history length does not affect much on XGaze~\cite{zhang2020eth} or MPIIGaze~\cite{zhang2017mpiigaze}. This is because neither of these datasets are free viewing tasks. Instead, participants will look at points/circles/pixels highlighted on screen and these points/circles/pixels are randomly sampled. In experiments, $\sim$1500 samples in MPIIGaze and $\sim$500 samples in XGaze would already cover most area on screen. 

%Our method is sensitive to history length for free viewing tasks such as those in EVE dataset. History of PoGs with low length does not guarantee to cover the common viewing area on screen, as a result, errors can occur when our Self-Calibration Module and Person-specific Transform Module digests this history to correct the current PoG. To investigate such effect, we conduct ablation studies on history length on EVE validation set. The results in Tab.~\ref{tbl:history_length_ablation_results_eve} show that the accuracy of our method improves with the increase of history length. 
%Our method performs the best with full history length (i.e., offline), averaged at 10817 for EVE validation set at 10Hz frame rate. Note that our method performs worse than InitNet (2.41$^{\circ}$) until the history length reaches 2000, so in we apply our online method to EVE validation and test set until the history length reaches 2000.

%In the main paper we tested our method on MPIIGaze using ResNet-preact-8 as InitNet~\cite{zhang2017mpiigaze}, which reduces the gaze direction error from 5.73$^{\circ}$ to 4.14$^{\circ}$. Here we applied our method using a better InitNet ResNet-14~\cite{zhang2017mpiigaze} and reduce the gaze direction error from 4.83$^{\circ}$ to 3.02$^{\circ}$. The proposed method achieved a $32.9\%$ improvement on MPIIGaze compared to the SOTA~\cite{park2018deep}. 

% ~\subsection{MPII results more}

% ~\subsection{XGaze results more}

%-------------------------------------------------------------------------
